# Supplementary material for: Mechanistic framework for reduced-order models in soft materials: Application to three-dimensional granular intrusion
Source: arXiv:2205.14920 ancillary file (2022-12-10)
Supplement: Supplementary file 1 [file SI-Mechanistic_framework_for_reduced_order_models_in_soft_materials__3DRFT.pdf]

1

## 2 **Supplementary Information for**

### 3 **Mechanistic framework for reduced-order models in soft materials: Application to** 4 **three-dimensional granular intrusion**

5 **Shashank Agarwal, Daniel I Goldman, Ken Kamrin**

6 **Ken Kamrin**

7 **E-mail: [kkamrin@mit.edu](mailto:kkamrin@mit.edu)**

#### 8 **This PDF file includes:**

- 9     Supplementary text
- 10    Figs. S1 to S8
- 11    Tables S1 to S4
- 12    SI References

## Supporting Information Text

### S1. Pre-existing 3D-RFT forms

The form of 3D-RFT proposed by Treers et al. (1) has the following formulation:

$$\mathbf{F} = \int_S \left[ f_1(\tilde{\psi}, \tilde{\gamma}) \alpha_y(\tilde{\gamma}, \tilde{\beta}) \hat{\mathbf{e}}_1 + f_{23}(\tilde{\psi}, \tilde{\gamma}) (-\alpha_x(\tilde{\gamma}, \tilde{\beta}) \hat{\mathbf{e}}_2 + \alpha_z(\tilde{\gamma}, \tilde{\beta}) \hat{\mathbf{e}}_3) \right] |z| dA \quad [1]$$

where the direction  $\hat{\mathbf{e}}_2$  represents the direction of the horizontal component of surface normal  $\hat{\mathbf{n}}$ ,  $\hat{\mathbf{e}}_3$  represents the vertical direction, and  $\hat{\mathbf{e}}_1$  represents the cross product of  $\hat{\mathbf{e}}_2$  and  $\hat{\mathbf{e}}_3$ . The angles  $\tilde{\beta}$ ,  $\tilde{\psi}$ , and  $\tilde{\gamma}$  characterize the plate and velocity directions in terms of basis directions  $\hat{\mathbf{e}}_1$ ,  $\hat{\mathbf{e}}_2$ , and  $\hat{\mathbf{e}}_3$ . We use a ‘~’ with these angles to differentiate them from the characteristic angles  $\beta$ ,  $\gamma$ , and  $\psi$  we use in the current work. Altogether,

$$\begin{aligned} \hat{\mathbf{e}}_3 &= \hat{\mathbf{z}} & \hat{\mathbf{e}}_2 &= \frac{\hat{\mathbf{n}} - (\hat{\mathbf{n}} \cdot \hat{\mathbf{z}}) \hat{\mathbf{z}}}{|\hat{\mathbf{n}} - (\hat{\mathbf{n}} \cdot \hat{\mathbf{z}}) \hat{\mathbf{z}}|} = \frac{(n_x, n_y, 0)}{\sqrt{n_x^2 + n_y^2}} & \hat{\mathbf{e}}_1 &= \hat{\mathbf{e}}_2 \times \hat{\mathbf{e}}_3 \\ \tilde{\gamma} &= \tan^{-1} \left( -\frac{\mathbf{v} \cdot \hat{\mathbf{e}}_3}{\mathbf{v} \cdot \hat{\mathbf{e}}_2} \right) = \tan^{-1} \left( -\frac{v_z \sqrt{n_x^2 + n_y^2}}{v_x n_x + v_y n_y} \right) & \tilde{\psi} &= \tan^{-1} \left( \frac{\mathbf{v} \cdot \hat{\mathbf{e}}_2}{\mathbf{v} \cdot \hat{\mathbf{e}}_1} \right) = \tan^{-1} \left( \frac{v_x n_x + v_y n_y}{v_x n_y - v_y n_x} \right) \\ \tilde{\beta} &= \tan^{-1} \left( \frac{n_z}{\sqrt{n_x^2 + n_y^2}} \right) - \frac{\pi}{2} \times \text{sign}(\hat{\mathbf{n}} \cdot \hat{\mathbf{z}}). \end{aligned}$$

The form was also used by Huang et al. (2) with a few minor modifications to the choices of the fittings functions  $f_1$  and  $f_{23}$ . We present two example cases of the limitations of this form, which show that in some situations it is too restrictive, while in others it is not restrictive enough.

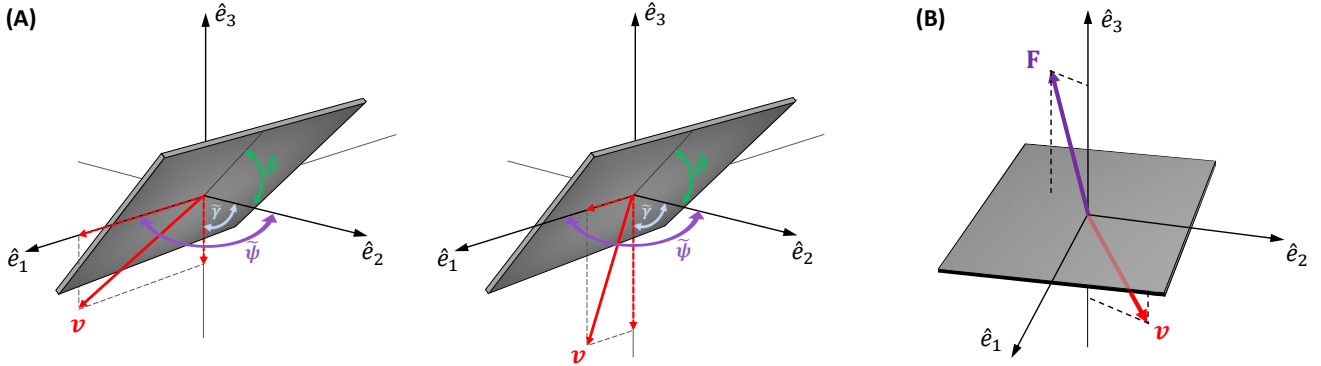

**Fig. S1. Pre-existing 3D-RFT verification:** (A) Case 1 — An example of an inappropriate system representation in pre-existing 3D-RFT. The two cases represent two different plate motions (same plate orientations but different velocity directions ( $\mathbf{v}$ ) in  $\hat{\mathbf{e}}_1 \hat{\mathbf{e}}_3$  plane), yet the form assigns identical characteristic angles ( $\tilde{\beta}$ ,  $\tilde{\gamma} = \pi/2$ ,  $\tilde{\psi} = \pi/2$ ) to define them. Thus, the 3D-RFT form predicts identical forces even though the two motions are expected to experience different resistive forces. (B) Case 2 — A plate oriented at  $\tilde{\beta} \rightarrow 0$ . The *global symmetry constraint* requires the force ( $\mathbf{F}$ ), the velocity ( $\mathbf{v}$ ), and the gravity ( $\mathbf{g}$ ) to be co-planar i.e.  $\mathbf{F}$  should lie in  $\mathbf{v}\mathbf{z}$  plane as shown in the figure as  $\tilde{\beta} \rightarrow 0$ . The pre-existing 3DRFT form does not satisfies this requirement.

In the first case, we consider a surface element oriented with a normal vector direction  $\hat{\mathbf{n}}$  and moving at a velocity  $\mathbf{v}$  such that  $\mathbf{v} \cdot \hat{\mathbf{e}}_2 = 0$ , i.e.  $v_x n_x + v_y n_y = 0$ . This corresponds to a velocity vector lying in the vertical plane that contains the horizontal tangent line of the plate. Based on the definitions above, this form of 3D-RFT requires the resistive force vector in this case to be independent of  $|v_z|$ . For example, a surface moving in any direction in the positive quadrant of the  $\hat{\mathbf{e}}_1 \hat{\mathbf{e}}_3$  plane is assumed to experience the same resistive force vector, since these motions always produce the same angles and same  $\hat{\mathbf{e}}$ 's. But this force response is not what is observed, nor what one would expect; using the angles defined in the main text, it corresponds to the proposition that the force does not change when varying  $\gamma$  at constant  $\beta$  and  $\psi = \pi/2$  but the reference data in Figure S8 show that in fact the force varies rather strongly with  $\gamma$ . Hence, this form of 3D-RFT in this case **over-constrains** the force response.

In the second case, we consider the IRT sub-constraint shown in Figure 3C of the main text which requires that in the limit of tilt approaching zero ( $\tilde{\beta} \rightarrow 0$ ), the force should lie in the  $\mathbf{v}\mathbf{z}$ -plane i.e.  $\lim_{\tilde{\beta} \rightarrow 0} (\mathbf{F} \cdot (\hat{\mathbf{v}} \times \hat{\mathbf{e}}_3)) = 0$  for all  $\tilde{\psi}$  and  $\tilde{\gamma}$ . Upon

substituting the above forms, we get:

$$\begin{aligned}
\mathbf{F} \cdot (\mathbf{v} \times \hat{\mathbf{e}}_3) &= \hat{\mathbf{e}}_3 \cdot (\mathbf{F} \times \mathbf{v}) = F_1 v_2 - F_2 v_1 \\
&= f_1(\tilde{\psi}, \tilde{\gamma}) \alpha_y(\tilde{\gamma}, \tilde{\beta}) |\mathbf{v} - (\mathbf{v} \cdot \hat{\mathbf{z}}) \hat{\mathbf{z}}| \cos \tilde{\psi} + f_{23}(\tilde{\psi}, \tilde{\gamma}) \alpha_x(\tilde{\gamma}, \tilde{\beta}) |\mathbf{v} - (\mathbf{v} \cdot \hat{\mathbf{z}}) \hat{\mathbf{z}}| \sin \tilde{\psi} \\
&= (f_1(\tilde{\psi}, \tilde{\gamma}) \alpha_y(\tilde{\gamma}, \tilde{\beta}) \cos \tilde{\psi} + f_{23}(\tilde{\psi}, \tilde{\gamma}) \alpha_x(\tilde{\gamma}, \tilde{\beta}) \sin \tilde{\psi}) \times |\mathbf{v} - (\mathbf{v} \cdot \hat{\mathbf{z}}) \hat{\mathbf{z}}| \\
&= (-f_1(\tilde{\psi}, \tilde{\gamma}) \alpha_x(0, 0) \cos \tilde{\psi} + f_{23}(\tilde{\psi}, \tilde{\gamma}) \alpha_x(\tilde{\gamma}, \tilde{\beta}) \sin \tilde{\psi}) \times |\mathbf{v} - (\mathbf{v} \cdot \hat{\mathbf{z}}) \hat{\mathbf{z}}| \quad [\text{Using } \alpha_y \text{ definition from Treers et al. (1)}] \\
&= (-f_1(\tilde{\psi}) \alpha_x(0, 0) \cos \tilde{\psi} + f_{23}(\tilde{\psi}) \alpha_x(\tilde{\gamma}, \tilde{\beta}) \sin \tilde{\psi}) \times |\mathbf{v} - (\mathbf{v} \cdot \hat{\mathbf{z}}) \hat{\mathbf{z}}|.
\end{aligned}$$

Note that we drop the  $\tilde{\gamma}$  dependence of  $f_1$  and  $f_{23}$  in the final step using the definitions from Treers et al. (1). Utilizing the fact that  $|\mathbf{v} - (\mathbf{v} \cdot \hat{\mathbf{z}}) \hat{\mathbf{z}}| = |\mathbf{v}|(1 + \tan^2 \tilde{\gamma} \cos^2 \tilde{\psi})^{-1/2}$  we obtain

$$\lim_{\tilde{\beta} \rightarrow 0} (\mathbf{F} \cdot (\hat{\mathbf{v}} \times \mathbf{e}_3)) = (-f_1(\tilde{\psi}) \alpha_x(0, 0) \cos \tilde{\psi} + f_{23}(\tilde{\psi}) \alpha_x(\tilde{\gamma}, 0) \sin \tilde{\psi}) (1 + \tan^2 \tilde{\gamma} \cos^2 \tilde{\psi})^{-1/2}$$

which is a non-trivial function of the two angles; it is not the zero function as it must be. The only way the expression above vanishes identically is if  $\alpha_x(\tilde{\gamma}, 0) = C$  and  $f_1(\tilde{\psi}) = C f_{23}(\tilde{\psi}) \tan \tilde{\psi} / \alpha_x(0, 0)$  for some constant  $C$ , which would be a very heavy-handed fit that would certainly not fit a range of data (and was not close to how those functions were fit in Treers et al. (1)). Thus, in this case, the chosen form **under-constrains** the force response and misses out on an important constraint the surface force response should follow.

## S2. Application of the 3-step procedure to other material models of soft media

The main text focuses on applying the general three-step procedure to deduce three-dimensional RFT for granular media. It is instructive to see how the methodology would be applied in other cases. This is primarily so for Steps 1 and 2, since the rotation symmetry of Step 3 is universal across all isotropic materials.

First of all, it bears noting that the quality of the approximation one obtains from a reduced-order intrusion model varies as one varies the underlying continuum model. In (3), a pseudo-diagnostic test was devised to assess the level of accuracy one might expect from the localization hypothesis (presumed in Step 1) as one varies the underlying rheological model. This so-called “garden hoe test” considers whether a localized rule for the surface stress,

$$\mathbf{F}^{\text{total}} = \int_{\text{surf}} \mathbf{t}(\hat{\mathbf{n}}, \mathbf{v}, \mathbf{g}, |z|; \text{mat}) ds \quad [2]$$

could possibly agree with full continuum-level solutions of the intrusion force. This test assesses the question by considering a very simple family of intruders — finite-sized square plates moving in arbitrary directions at arbitrary tilts. What varies as one changes the rheological model is the parameter set invoked by *mat*. In frictional media, as in the main text,  $\text{mat} = \{\rho_c, \mu_s, \mu_w\}$ ; in purely cohesive solids  $\text{mat} = \{\rho, \sigma_y\}$  for yield stress  $\sigma_y$ ; in viscous fluids  $\text{mat} = \{\rho, \eta\}$  for viscosity  $\eta$ ; in inviscid (Euler) fluids  $\text{mat} = \{\rho\}$ ; and so on. For each *mat*, dimensional analysis and physical constraints of the continuum PDE’s put strong restrictions on how the surface traction formula  $\mathbf{t}(\cdot)$  is allowed to depend on its inputs. To deduce if a material “passes” the garden hoe test, one uses this constrained form for the  $\mathbf{t}(\cdot)$  function to infer the resistive force on a finite-sized square intruding plate and then compares this answer to a known full-field result from the continuum theory. Some material models pass the garden hoe test — the localized force formula agrees exactly with the result one would obtain from the full continuum solution — while others do not. For example, frictional media, purely cohesive solids, and inviscid fluids pass the test, but viscous fluids do not. Interestingly, we have observed that materials which pass the garden hoe test also happen to display a strong collapse to the RFT approximation in general, that is, when non-rectangular intruders are used (3). We do not have a complete proof for this.

In contrast to cohesionless grains, gravity and intruder depth play a smaller role in intrusion problems in media with pressure-insensitive shear stress (aside from a standard buoyancy term). We show three examples next in this limit, where possible dependence on  $|z|$  and  $\mathbf{g}$  is neglected.

For cohesive materials with a constant rate-independent yield stress, such as muds or foams in a certain slow limit, the corresponding RFT-like rule after Steps 1 and 2 is

$$\text{Cohesive media:} \quad \mathbf{t} = \sigma_y \mathbf{a}^{\text{gen}}(\hat{\mathbf{n}}, \hat{\mathbf{v}})$$

for some dimensionless universal function  $\mathbf{a}^{\text{gen}}(\cdot)$ . The form for the traction shown above is the only dimensionally sound formula for the given material property set in the slow limit. And when the above relation is tested in non-flat-plate intrusion tests and compared to full-field results, a high-level agreement is observed (3) indicative of strong general accuracy of the reduced-order RFT formula.

Unlike the previous examples, which are considered in the inertialess limit, for inviscid fluids the intrusion force arises solely from the inertia transferred to the fluid. Hence, in this case, after Step 2, one has the following dimensionally-sound local traction form

$$\text{Inviscid fluid:} \quad \mathbf{t} = \rho v^2 \mathbf{b}^{\text{gen}}(\hat{\mathbf{n}}, \hat{\mathbf{v}})$$

for some dimensionless universal function  $\mathbf{b}^{\text{gen}}(\cdot)$ . The resulting form produces an accurate model for locomotion of swimming centipedes (4) and has been indirectly validated through the success of the so-called “Blade Element Theory” of rotor design (5), which uses a similar localization rule to determine drag and lift forces for generically shaped rotors moving through an inviscid fluid.

In materials that do not pass the garden hoe test, we can still obtain a best possible approximate reduced-order model for intrusion, even if its accuracy may never rise to the level seen in frictional or cohesive media. In these cases, additional information can be used to obtain an approximate localization rule. A useful case in point is viscous media, which does not pass the garden hoe test because the force on an intruding square plate of size  $L$  in a large domain of viscous media must have the form

$$\mathbf{F}^{\text{total}} = L\eta v \mathbf{c}^{\text{gen}}(\hat{\mathbf{n}}, \hat{\mathbf{v}})$$

for some dimensionless function  $\mathbf{c}^{\text{gen}}(\cdot)$ . The linearity in  $v$  is required due to linearity in the Stokes equations. Since the force does not scale as  $L^2$  a localized superposition rule of the form of Eq. (2) will not be precise even for simple plate intruders. However, and as is the tradition for viscous RFT going back to Gray and Hancock (6), one can assert an additional length-scale  $\lambda$  within the force model to obtain an approximate form. One can use the entire diameter of the immersed object as  $\lambda$ , or, in the case of viscous quasi-1D swimmers, one often uses the wavelength of the swimming mode. However it is chosen, we can then write the quasi-local form for the mean traction on a plate of size  $\lambda$  in viscous fluid as

$$\text{Viscous fluid:} \quad \mathbf{t} = \frac{\eta v}{\lambda} \mathbf{c}^{\text{gen}}(\hat{\mathbf{n}}, \hat{\mathbf{v}})$$

Utilizing this relation in Eq. (2) gives a result that only matches the exact solution for a finite plate in the case that the plate has a size of  $L = \lambda$ . However, even when this is not the case, the formula can still be used as an approximation.

### S3. Verification of leading edge hypothesis in 3D-RFT

We verify the applicability of the ‘leading-edge hypothesis’ (ie., the assumption that no force occurs on surfaces with  $\mathbf{n} \cdot \mathbf{v} \leq 0$ ) during three-dimensional plate motion. To verify the hypothesis, we plot the variations of forces on the front and the back surface-nodes of the plate geometry used for generating the reference 3D-RFT graphs. Figure S2 shows the variations of force magnitudes on the two surfaces the plates used for modeling intrusions. We plot these results for six plate and velocity configurations. The sides are color-coded in blue and red. In the first two cases, the front-face (in red) acts as the leading edge. In the next two cases, the back-face (in blue) acts as the leading edge. In all such cases, we measure leading edges forces, as non-leading edge forces are negligible in comparison to leading-edge forces. In the last two cases, both the faces experience equal force magnitudes with (equal tangential forces but equal and opposite normal forces). The last two cases correspond to the slicing motion of the surfaces. We take average force magnitudes for making RFT plots in such cases. We observed similar behavior in other plate and velocity configurations.

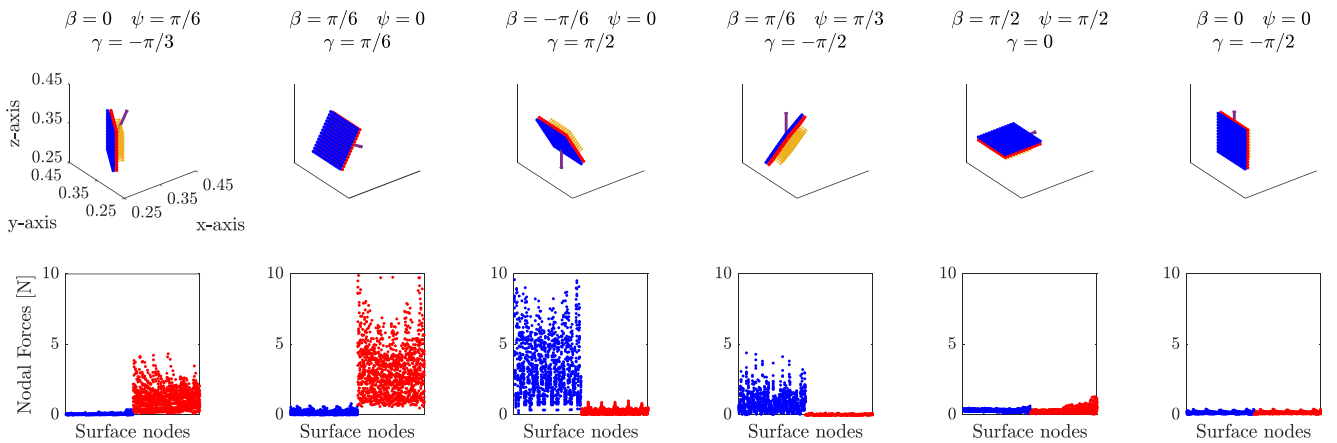

**Fig. S2. Leading edge hypothesis verification::** Variation of the magnitude of forces on the two sides of thin plates during granular intrusions. The sides are color-coded in blue and red. The yellow arrows show front-face normals, and the violet arrow shows the velocity direction. We plot six combinations of plate configurations and velocity directions. In the first two cases, the front-face (in red) acts as the leading edge. In the next two cases, the back-face (in blue) acts as the leading edge. And in the last two cases, both the faces experience equal force magnitudes with (equal tangential forces but equal and opposite normal forces). The last two cases correspond to the slicing motion of the surfaces. We take average force magnitudes for making RFT plots in such cases.

88

### S4. Reference data generation; internal friction ( $\mu_{\text{int}}$ ) dependence of 3D-RFT

We use a large combination of material properties ( $\rho_c, \mu_{\text{int}}, \mu_{\text{surf}}$ ) and 3D-RFT reference variables ( $\beta, \gamma, \psi$ ) to generate continuum modeling-based reference data for evaluating the 3D-RFT form. In regards to the material properties we use five material

91

internal friction values ( $\mu_{\text{int}} = [0.3, 0.4, 0.5, 0.7, 0.9]$ ) with two values of surface friction ( $\mu_{\text{surf}}$ ) in each case. For  $\mu_{\text{int}} = 0.4$  we use 3 instead of 2  $\mu_{\text{surf}}$  values. For each of the 11 combinations of  $\mu_{\text{int}}$  and  $\mu_{\text{surf}}$ , we conduct plate intrusions at 7 combinations of plate tilt angle ( $\beta = -\pi/2 : \pi/6 : \pi/2$  rad), 7 combinations of velocity direction angle ( $\gamma = -\pi/2 : \pi/6 : \pi/2$  rad), and 4 combinations of plate twist angle ( $\psi = 0 : \pi/6 : \pi/2$  rad). For the  $\{\mu_{\text{int}} = 0.40, \mu_{\text{surf}} = 0.15\}$ , we use 13 combinations of  $\beta$  ( $\pi/2 : \pi/6 : \pi/2$  rad), 13 combinations of  $\gamma$  ( $-\pi/2 : \pi/6 : \pi/2$  rad), and 4 combinations of  $\psi$  ( $0 : \pi/6 : \pi/2$  rad). Additionally, we conduct plate intrusion simulations at  $\{\mu_{\text{int}} = 0.2, \mu_{\text{surf}} = 0.2\}$  and  $\{\mu_{\text{int}} = 0.1, \mu_{\text{surf}} = 0.1\}$  at  $\psi = 0$  rad to evaluate  $\xi_n$  at  $\mu_{\text{int}} = 0.1$  and  $0.2$ . We do not explore  $\psi$  in  $[-\pi/2 : 0]$  rad range for the reference data as  $\alpha_r$ ,  $\alpha_z$ , and  $\alpha_\theta$  are known to be even, even, and odd (resp.) in  $\psi$  from ‘plate twist symmetry’. The polynomial fits for  $f_1$ ,  $f_2$ , and  $f_3$  are provided in Tables S3 and S4.

We explore the dependence of 3D-RFT forces on material internal friction by conducting plate intrusion simulations for five different values of ( $\mu_{\text{int}}$ ) at two values of surface friction ( $\mu_{\text{surf}}$ ) each (except  $\mu_{\text{int}} = 0.4$  for which we explore 3 values of  $\mu_{\text{surf}}$ ). To better understand the trends in variations of  $\alpha$ , we only consider the normal component of  $\alpha$  i.e.  $\alpha_n$ . Figure S3 shows values of  $\alpha_n$  scaled by the scaling coefficient  $\xi_n$ . These plots show that  $\xi_n$  primarily depends on  $\mu_{\text{int}}$  (in addition to its linear dependence of  $\rho_c$  and  $g$ , i.e.  $\xi_n = \rho_c g \hat{f}(\mu_{\text{int}})$ ). Figure S4 shows the variation of  $\xi_n / \rho_c g$  with  $\mu_{\text{int}}$ . This figure uses two additional values of  $\mu_{\text{int}}$  — 0.1 and 0.2. We conducted additional simulations at limited  $\mu_{\text{surf}}$  and  $\psi$  for these  $\mu_{\text{int}}$ ’s for better understandings the  $\xi_n$  vs  $\mu_{\text{int}}$  trends, as discussed in Materials and Methods section. We find superlinear dependence of  $\xi_n$  on  $\mu_{\text{int}}$ , which was also observed by researchers (7). Figure S4 can be used for interpreting the value of  $\xi_n$  from  $\rho_c$ ,  $g$ , and  $\mu_{\text{int}}$  (or the angle of repose,  $\theta = \tan^{-1}(\mu_{\text{int}})$ ) of a non-cohesive granular media. Exact values of  $\xi_n$  and  $\mu_{\text{int}}$  corresponding to Figure S4 are given in Table S1.

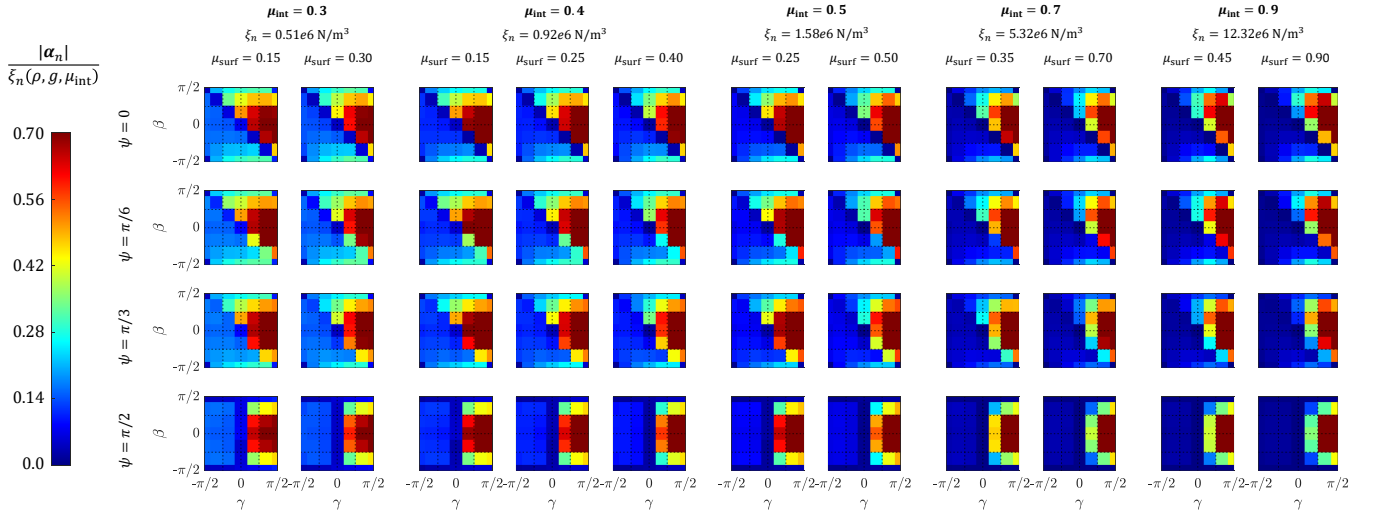

**Fig. S3.** Variation of  $\alpha_n$  with  $\mu_{\text{int}}$ : Variation of normal component of stress/depth (scaled by  $\xi_n$ ) for various combinations of  $\mu_{\text{int}}$  and  $\mu_{\text{surf}}$ . The variations of normalized  $\xi_n$  with  $\mu_{\text{int}}$  are plotted in figure S4. Corresponding values of  $\mu_{\text{int}}$ ,  $\mu_{\text{surf}}$ , and  $\xi_n$  are written at the top of each column. The granular material had an effective density of ( $\rho_c$ ) 3000 kg/m<sup>3</sup> in the cases.

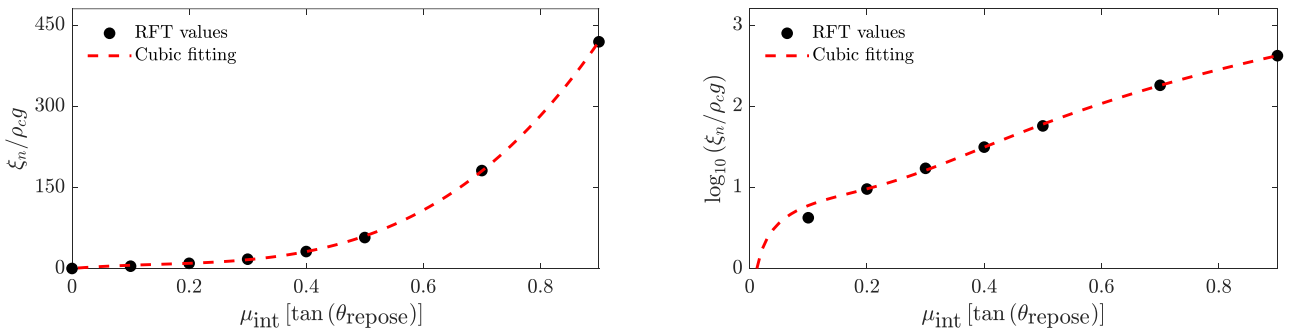

**Fig. S4.** Variation of  $\xi_n$  with material properties: Variation of normalized scaling coefficient  $\xi_n$  (normalized with density  $\rho_c$  and gravity  $g$ ) with material internal coefficient of friction ( $\mu_{\text{int}}$ ) on (A) linear and (B) logarithmic scale. The cubic fitting (red dotted lines) is  $\xi_n^{\text{fit}} = \rho_c g (894\mu_{\text{int}}^3 - 386\mu_{\text{int}}^2 + 89\mu_{\text{int}})$ . Corresponding values are given in table S1.

**Table S1. Variation of  $\xi_n$  with  $\mu_{\text{int}}$  at  $\rho_c = 3000 \text{ kg/m}^3$**

| $\mu_{\text{int}}$ | $\theta_{\text{repose}} [^\circ]$ | $\xi_n [\times 10^6 \text{ N/m}^3]$ |
|--------------------|-----------------------------------|-------------------------------------|
| 0.0                | $0^\circ$                         | 0.0                                 |
| 0.1                | $5.7^\circ$                       | 0.13                                |
| 0.2                | $11.3^\circ$                      | 0.28                                |
| 0.3                | $16.7^\circ$                      | 0.51                                |
| 0.4                | $21.8^\circ$                      | 0.92                                |
| 0.5                | $26.5^\circ$                      | 1.58                                |
| 0.7                | $35.0^\circ$                      | 5.32                                |
| 0.9                | $42.0^\circ$                      | 12.32                               |

## 111 S5. Surface friction ( $\mu_{\text{surf}}$ ) dependence of 3D-RFT

112 Similar to  $\mu_{\text{int}}$ , we explore the dependence of 3D-RFT forces on material-body surface friction ( $\mu_{\text{surf}}$ ) by conducting plate  
 113 intrusions at different combinations of  $\mu_{\text{int}}$  and  $\mu_{\text{surf}}$ . To better understand the trends, we consider the ratio of the normal and  
 114 tangential components of  $\alpha$  i.e.  $|\alpha_t|/|\alpha_n|$ . Figure S5 shows values of  $\alpha_n$  scaled by the scaling coefficient  $\xi_n$  discussed in the  
 115 previous section and shown in figure S4. The plots show that the ratio  $|\alpha_t|/|\alpha_n|$  largely remains independent of  $\mu_{\text{int}}$  as the  
 116 graphs remain largely identical for same values of  $\mu_{\text{surf}}$  at different values of  $\mu_{\text{int}}$ . We also see that for  $\mu_{\text{surf}}^{(1)} < \mu_{\text{surf}}^{(2)}$ , the graph  
 117 for the lower surface friction case appears to be obtainable from the graph at the higher friction by way of a simple cut-off that  
 118 ensures non-violation of the Coulomb condition based on  $\mu_{\text{surf}}^{(1)}$ . Equation 7 incorporates this concept into the final form of  
 119 3D-RFT. The proposed generic 3D-RFT graphs in this study correspond to  $\mu_{\text{surf}} = 0.9$ .

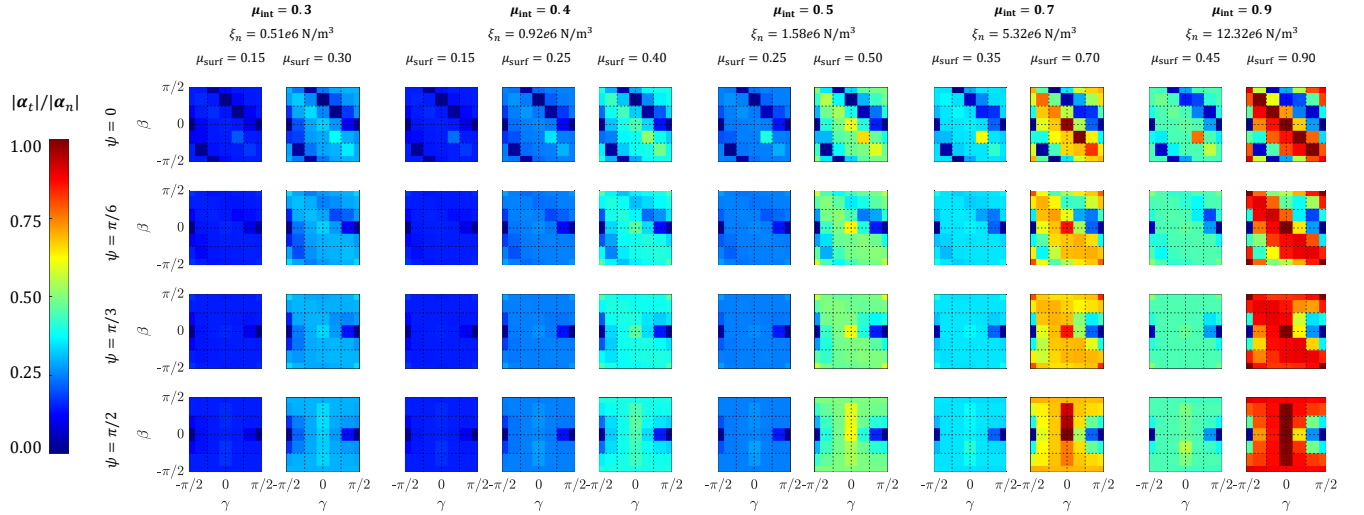

**Fig. S5. Variation of  $|\alpha_t|/|\alpha_n|$  with material properties:** Variation of ratio of magnitude of  $\alpha$  in tangential and normal directions. The ratio never exceeds the individual  $\mu_{\text{surf}}$  values in each case due to the Coulomb friction condition. Corresponding values of  $\mu_{\text{int}}$ ,  $\mu_{\text{surf}}$ , and  $\xi_n$  are written at the top of each column. The granular material used has an effective density of ( $\rho_c$ )  $3000 \text{ kg/m}^3$ .

## 120 S6. Proof that Coulomb friction cut-off does not affect satisfaction of global rotational symmetry constraint

Given that  $\alpha^{\text{gen}}$  obeys Eq 6 and thus satisfies the global rotation constraint, we want to prove that  $\alpha$  as represented in Eq 5 for general internal and surface frictions also obeys the global rotation constraint. First, we notice that if  $\alpha^{\text{gen}}$  obeys the rotational symmetry constraint then  $\alpha_n^{\text{gen}} = \alpha^{\text{gen}} \cdot \hat{n}$  and  $\alpha_t^{\text{gen}} = \alpha^{\text{gen}} - (\alpha^{\text{gen}} \cdot \hat{n}) \hat{n}$  must also obey the rotational symmetry

constraint. Under an arbitrary rotation  $\mathbf{R}$  of the inputs, Eq 5 imply

$$\begin{aligned}
& \alpha(\mathbf{R}\hat{\mathbf{n}}, \mathbf{R}\hat{\mathbf{v}}, \mathbf{R}\hat{\mathbf{g}}; \rho_c, \mu_{\text{int}}, \mu_{\text{surf}}) \\
&= \rho_c g \hat{f}(\mu_{\text{int}}) |\alpha_n^{\text{gen}}(\mathbf{R}\hat{\mathbf{n}}, \mathbf{R}\hat{\mathbf{v}}, \mathbf{R}\hat{\mathbf{g}})| \hat{\mathbf{n}} + \rho_c g \hat{f}(\mu_{\text{int}}) \min \left( \frac{\mu_{\text{surf}} |\alpha_n^{\text{gen}}(\mathbf{R}\hat{\mathbf{n}}, \mathbf{R}\hat{\mathbf{v}}, \mathbf{R}\hat{\mathbf{g}})|}{|\alpha_t^{\text{gen}}(\mathbf{R}\hat{\mathbf{n}}, \mathbf{R}\hat{\mathbf{v}}, \mathbf{R}\hat{\mathbf{g}})|}, 1 \right) \alpha_t^{\text{gen}}(\mathbf{R}\hat{\mathbf{n}}, \mathbf{R}\hat{\mathbf{v}}, \mathbf{R}\hat{\mathbf{g}}) \\
&= \rho_c g \hat{f}(\mu_{\text{int}}) |\mathbf{R}\alpha_n^{\text{gen}}(\hat{\mathbf{n}}, \hat{\mathbf{v}}, \hat{\mathbf{g}})| \mathbf{R}\hat{\mathbf{n}} + \rho_c g \hat{f}(\mu_{\text{int}}) \min \left( \frac{\mu_{\text{surf}} |\mathbf{R}\alpha_n^{\text{gen}}(\hat{\mathbf{n}}, \hat{\mathbf{v}}, \hat{\mathbf{g}})|}{|\mathbf{R}\alpha_t^{\text{gen}}(\hat{\mathbf{n}}, \hat{\mathbf{v}}, \hat{\mathbf{g}})|}, 1 \right) \mathbf{R}\alpha_t^{\text{gen}}(\hat{\mathbf{n}}, \hat{\mathbf{v}}, \hat{\mathbf{g}}) \\
&= \mathbf{R} \rho_c g \hat{f}(\mu_{\text{int}}) |\alpha_n^{\text{gen}}(\hat{\mathbf{n}}, \hat{\mathbf{v}}, \hat{\mathbf{g}})| \hat{\mathbf{n}} + \rho_c g \hat{f}(\mu_{\text{int}}) \min \left( \frac{\mu_{\text{surf}} |\alpha_n^{\text{gen}}(\hat{\mathbf{n}}, \hat{\mathbf{v}}, \hat{\mathbf{g}})|}{|\alpha_t^{\text{gen}}(\hat{\mathbf{n}}, \hat{\mathbf{v}}, \hat{\mathbf{g}})|}, 1 \right) \alpha_t^{\text{gen}}(\hat{\mathbf{n}}, \hat{\mathbf{v}}, \hat{\mathbf{g}}) \\
&= \mathbf{R}\alpha(\hat{\mathbf{n}}, \hat{\mathbf{v}}, \hat{\mathbf{g}}; \rho_c, \mu_{\text{int}}, \mu_{\text{surf}})
\end{aligned} \tag{3}$$

121 Thus, the 3D-RFT form in Eq 5 continues to satisfy IRT requirements and thus satisfy the global rotational constraint.

## 122 S7. 3D-RFT Implementation

We use an explicit iterative scheme to implement 3D-RFT in this study. The strategy primarily consists three parts — (1) discretizing the intruder surface into small sub-surfaces, (2) finding the sub-surface forces using sub-surface orientation angles ( $\beta$  and  $\psi$ ), velocity angle ( $\gamma$ ), area ( $ds$ ), and depth from the free surface ( $|z|$ ), and (3) summing over all sub-surfaces to find the net resistive force and moment response. A step-by-step implementation of the strategy is provided below:

**Step 1:** Discretize the intruder surface into small plane sub-surface elements. We use the open-source software, ‘Blender’ (version 2.91) for modeling and discretizing various intruder geometries in our study (using .wrl format).

**Step 2:** Calculate the velocity direction vector  $\hat{\mathbf{v}}$ , surface normal  $\hat{\mathbf{n}}$ , and depth from the free surface  $|z|$  for each sub-surface. Repeat Steps 3-11 for each sub-surface.

**Step 3:** Check if  $\hat{\mathbf{n}} \cdot \hat{\mathbf{v}} \geq 0$  (sub-surface is a ‘leading edge’) and  $z < 0$  (sub-surface is submerged in the media). If both the conditions are met, follow Steps 4-11. If they are not, set the sub-surface resistive force to zero and consider the next sub-surface. Also, the application of 3D-RFT is limited to  $|z| < O(10)L$  where  $L$  is the characteristic length of the intruder. RFT is (especially vertical force) expected to over-predict intrusion forces beyond this limit.

**Step 4:** Find local coordinate frame  $\{\hat{\mathbf{r}}, \hat{\boldsymbol{\theta}}, \hat{\mathbf{z}}\}$  using following relations:

$$\hat{\mathbf{z}} = -\hat{\mathbf{g}} \quad \hat{\mathbf{r}} = \frac{\mathbf{v} - (\mathbf{v} \cdot \hat{\mathbf{z}})\hat{\mathbf{z}}}{|\mathbf{v} - (\mathbf{v} \cdot \hat{\mathbf{z}})\hat{\mathbf{z}}|} \quad \hat{\boldsymbol{\theta}} = \hat{\mathbf{z}} \times \hat{\mathbf{r}} \tag{4}$$

When  $|\mathbf{v} - (\mathbf{v} \cdot \hat{\mathbf{z}})\hat{\mathbf{z}}|$  is zero (a sub-surface moves up or down),  $\hat{\mathbf{r}}$  is set to the direction of horizontal component of the surface-normal i.e.  $\hat{\mathbf{r}} = (\hat{\mathbf{n}} - (\hat{\mathbf{n}} \cdot \hat{\mathbf{z}})\hat{\mathbf{z}})/|\hat{\mathbf{n}} - (\hat{\mathbf{n}} \cdot \hat{\mathbf{z}})\hat{\mathbf{z}}|$ .

**Step 5:** Find RFT characteristic angles  $\{\beta, \gamma, \psi\}$  using  $\{\hat{\mathbf{v}}, \hat{\mathbf{g}}, \hat{\mathbf{n}}\}$  and local coordinate frame  $\{\hat{\mathbf{r}}, \hat{\boldsymbol{\theta}}, \hat{\mathbf{z}}\}$  as follows:

Find the surface characteristic angle  $\beta$  as:

$$\begin{aligned}
\beta = & \begin{aligned} & -\cos^{-1}(\hat{\mathbf{n}} \cdot \hat{\mathbf{z}}) & \text{if } \hat{\mathbf{n}} \cdot \hat{\mathbf{r}} \geq 0 \quad \& \quad \hat{\mathbf{n}} \cdot \hat{\mathbf{z}} \geq 0 \\ & +\pi - \cos^{-1}(\hat{\mathbf{n}} \cdot \hat{\mathbf{z}}) & \text{if } \hat{\mathbf{n}} \cdot \hat{\mathbf{r}} \geq 0 \quad \& \quad \hat{\mathbf{n}} \cdot \hat{\mathbf{z}} < 0 \\ & \cos^{-1}(\hat{\mathbf{n}} \cdot \hat{\mathbf{z}}) & \text{if } \hat{\mathbf{n}} \cdot \hat{\mathbf{r}} < 0 \quad \& \quad \hat{\mathbf{n}} \cdot \hat{\mathbf{z}} \geq 0 \\ & -\pi + \cos^{-1}(\hat{\mathbf{n}} \cdot \hat{\mathbf{z}}) & \text{if } \hat{\mathbf{n}} \cdot \hat{\mathbf{r}} < 0 \quad \& \quad \hat{\mathbf{n}} \cdot \hat{\mathbf{z}} < 0 \end{aligned}
\end{aligned} \tag{5}$$

Remember that this  $\beta$  corresponds to only ‘leading edges’ as non ‘leading-edge’ sub-surface never reach this step.

Find the velocity characteristic angle  $\gamma$  as:

$$\begin{aligned}
\gamma = & \begin{aligned} & \cos^{-1}(\hat{\mathbf{v}} \cdot \hat{\mathbf{r}}) & \text{if } \hat{\mathbf{v}} \cdot \hat{\mathbf{z}} \leq 0 \\ & -\cos^{-1}(\hat{\mathbf{v}} \cdot \hat{\mathbf{r}}) & \text{if } \hat{\mathbf{v}} \cdot \hat{\mathbf{z}} \geq 0 \end{aligned}
\end{aligned} \tag{6}$$

Find the surface characteristic angle  $\psi$  as:

$$\begin{aligned}
\psi = & \tan^{-1}((\hat{\mathbf{n}}_{r\theta} \cdot \hat{\mathbf{r}})/(\hat{\mathbf{n}}_{r\theta} \cdot \hat{\mathbf{r}})) \\
\text{where, } \hat{\mathbf{n}}_{r\theta} = & \frac{\hat{\mathbf{n}} - (\hat{\mathbf{n}} \cdot \hat{\mathbf{z}})\hat{\mathbf{z}}}{|\hat{\mathbf{n}} - (\hat{\mathbf{n}} \cdot \hat{\mathbf{z}})\hat{\mathbf{z}}|}
\end{aligned} \tag{7}$$

If  $|\hat{n} - (\hat{n} \cdot \hat{z})\hat{z}| = 0$ , set  $\psi = 0$ . In case both  $\hat{v}$  and  $\hat{n}$  align to  $\hat{z}$  ( $\gamma = \pm\pi/2$  and  $\psi = 0$ ), set  $\hat{r}$  in global  $x$ -direction.

**Step 6:** Calculate  $\{\hat{g} \cdot \hat{v}, \hat{g} \cdot \hat{n}, \hat{n} \cdot \hat{v}\}$  using Eq 8 of the main text as:

$$\hat{g} \cdot \hat{v} = \sin \gamma, \quad \hat{g} \cdot \hat{n} = \cos \beta, \quad \hat{n} \cdot \hat{v} = \cos \psi \cos \gamma \sin \beta + \sin \gamma \cos \beta \quad [8]$$

and calculate  $f_1, f_2, f_3$  using their dependencies on  $\{\hat{g} \cdot \hat{v}, \hat{g} \cdot \hat{n}, \hat{n} \cdot \hat{v}\}$  from table S3 (or table S4). Note that these equations use following expressions of  $\{\hat{n}, \hat{v}, \hat{g}\}$  in  $\{\hat{r}, \hat{\theta}, \hat{z}\}$  coordinate frame:

$$\hat{g} = -\hat{z}, \quad \hat{v} = \cos \gamma \hat{r} - \sin \gamma \hat{z}, \quad \hat{n} = \sin \beta \cos \psi \hat{r} + \sin \beta \sin \psi \hat{\theta} - \cos \beta \hat{z}. \quad [9]$$

**Step 7:** Calculate the values of  $\{\alpha_r^{\text{gen}}, \alpha_\theta^{\text{gen}}, \alpha_z^{\text{gen}}\}$  using Eq 9 (of the main text) and table S3 (or table S4).

**Step 8:** Estimate the media specific scaling factor  $\xi_n (= \rho_c g \hat{f}(\mu_{\text{int}}))$  using expected functional form of  $\xi_n$  from Table S1 and Fig S3 of the Supplementary Information if the media effective density ( $\rho_c$ ), gravity magnitude ( $g$ ), and media internal friction coefficient ( $\mu_{\text{int}}$ ) are known. Alternatively, obtain  $\xi_n$  from vertical plate intrusion experiments (intrusion of a thin flat plate of area  $ds$  at  $\beta = 0$ ,  $\psi = 0$ , and  $\gamma = \pi/2$ ) using the following formula:

$$\xi_n = \frac{F_{\text{vertical}}}{\alpha_z^{\text{gen}}(\beta = 0, \gamma = \pi/2, \psi = 0) \times ds \times |z|} \quad [10]$$

where,  $|z|$  corresponds to the average depth of the plate from the free surface at which the force is measured.

**Step 9:** Calculate the sub-surface(s) specific  $\alpha_n^{\text{gen}}$  and  $\alpha_t^{\text{gen}}$  in the local coordinates (from the values of  $\alpha_{r,\theta,z}^{\text{gen}}$  and  $\hat{n}$ ) and add them up using Eq 5 of the main text to get  $\alpha$ .

**Step 10:** Calculate  $\{\alpha_x, \alpha_y, \alpha_z\}$  by substituting triad  $\{\hat{r}, \hat{\theta}, \hat{z}\}$  from step 4.

**Step 11:** Calculate the net resistive force on the sub-surface by multiplying the triad  $\{\alpha_x, \alpha_y, \alpha_z\}$  with sub-surface depth ( $|z_i|$ ), and area ( $ds_i$ )

**Step 12:** Sum over all the sub-surfaces to find the net force and moment on the intruder.

Once the net resistive force on the intruder is known, one can use momentum balance equations to further model the intruder motion. Convergence studies are also done to determine the discretization of the intruder shape.

## S8. DEM simulations

In this section, we discuss the details of DEM systems used for verifications studies. We use DEM based LIGGGHTS package for modeling grains. We use a 50/50 split of 3.0 mm and 3.4 mm diameter ( $d$ ) grains in all the DEM simulations. More material properties are given in table S2. We use a simple shear simulation setup to determine the internal friction of the bulk of the granular volume. The setup consisted of a  $100d \times 50d \times 90d$  granular bed in plane-strain condition and was sheared with rigid plates on the top and the bottom as shown in figure S6. For uniform shearing at constant pressure, a uniformly distributed constant force ( $F_{\text{top}}$ ) was applied on the top plate whose motion was restricted to  $z$ -direction. An identical bottom plate was moved in positive  $x$ -direction to create the quasi-static simple shear condition.

**Table S2. DEM material properties**

|                                     |                                  |
|-------------------------------------|----------------------------------|
| Grain diameter ( $d$ )              | 50/50 split: 3 mm / 3.4 mm       |
| Grain density ( $\rho_g$ )          | 2470 kg/m <sup>3</sup>           |
| Packing efficiency ( $\phi$ )       | $\sim 0.59$                      |
| Contact model                       | Hookean contact model            |
| Elastic modulus, $E$                | $7 \times 10^6$ N/m <sup>2</sup> |
| Poisson's ratio, $\nu$              | 0.45                             |
| Coefficient of restitution, $e$     | 0.88                             |
| Grain-grain friction, $\mu_{g-g}$   | 0.05                             |
| Grain-surface friction, $\mu_{g-s}$ | 0.4                              |
| Characteristic velocity             | 2                                |

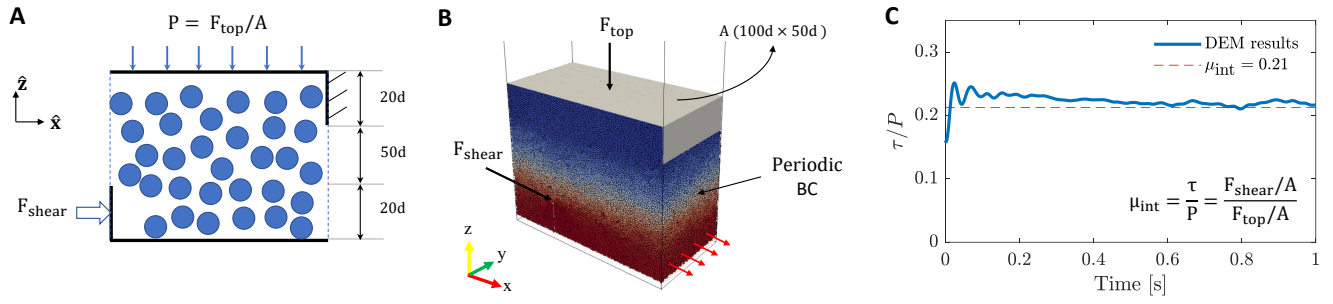

**Fig. S6.** Simple shear DEM setup: (A) 2D schematic and (B) 3D snapshot of the DEM simulation setup used for finding the internal friction coefficient of DEM particles used for verification studies. (C) Variation of the ratio of shear stress ( $\tau = F_{shear}/A$ ) and pressure ( $P = F_{top}/A$ ) as a function of time from DEM (solid blue line) and fitted estimate (red dotted line). Material properties are provided in table S2

**Radius of curvature corrections to DEM Bunny drill simulations:** As discussed in 3D-RFT premises, the RFT form assumes a scale separation by treating granular media as a continua. This assumption limits the performance of 3D-RFT when objects have sharp corners. While characterizing these effects would be a work for the future, we attempt to incorporate these effects at the most basic level in bunny drill simulations. This is important in the Bunny drill case especially because many features of the bunny shape have competing length scales to grain size in this DEM-based study. The grain size could not be reduced further in this study due to limitations on computational resources. Thus, we use a simple *Radius of curvature* ( $R_c$ ) based identification of low- $R_c$  regions of this intruder. We assume that any surface with a vertex with a radius of curvature lesser than 2 times the average grain radius will not experience any resistive force from the granular volumes.  $R_c$  was calculated using the discrete principle curvature formula from Hao Li's lecture notes (8). Figure S7 shows the radius of curvature estimation across the bunny shape used in this study.

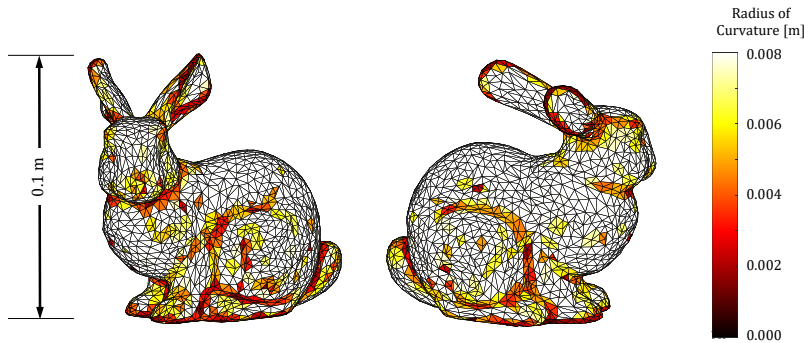

**Fig. S7.** Variation of radius of curvature ( $R_c$ ) on Bunny shape: The colormap on the right shows the variations.  $R_c$  cut-off for active surfaces was set at 0.0048 m.

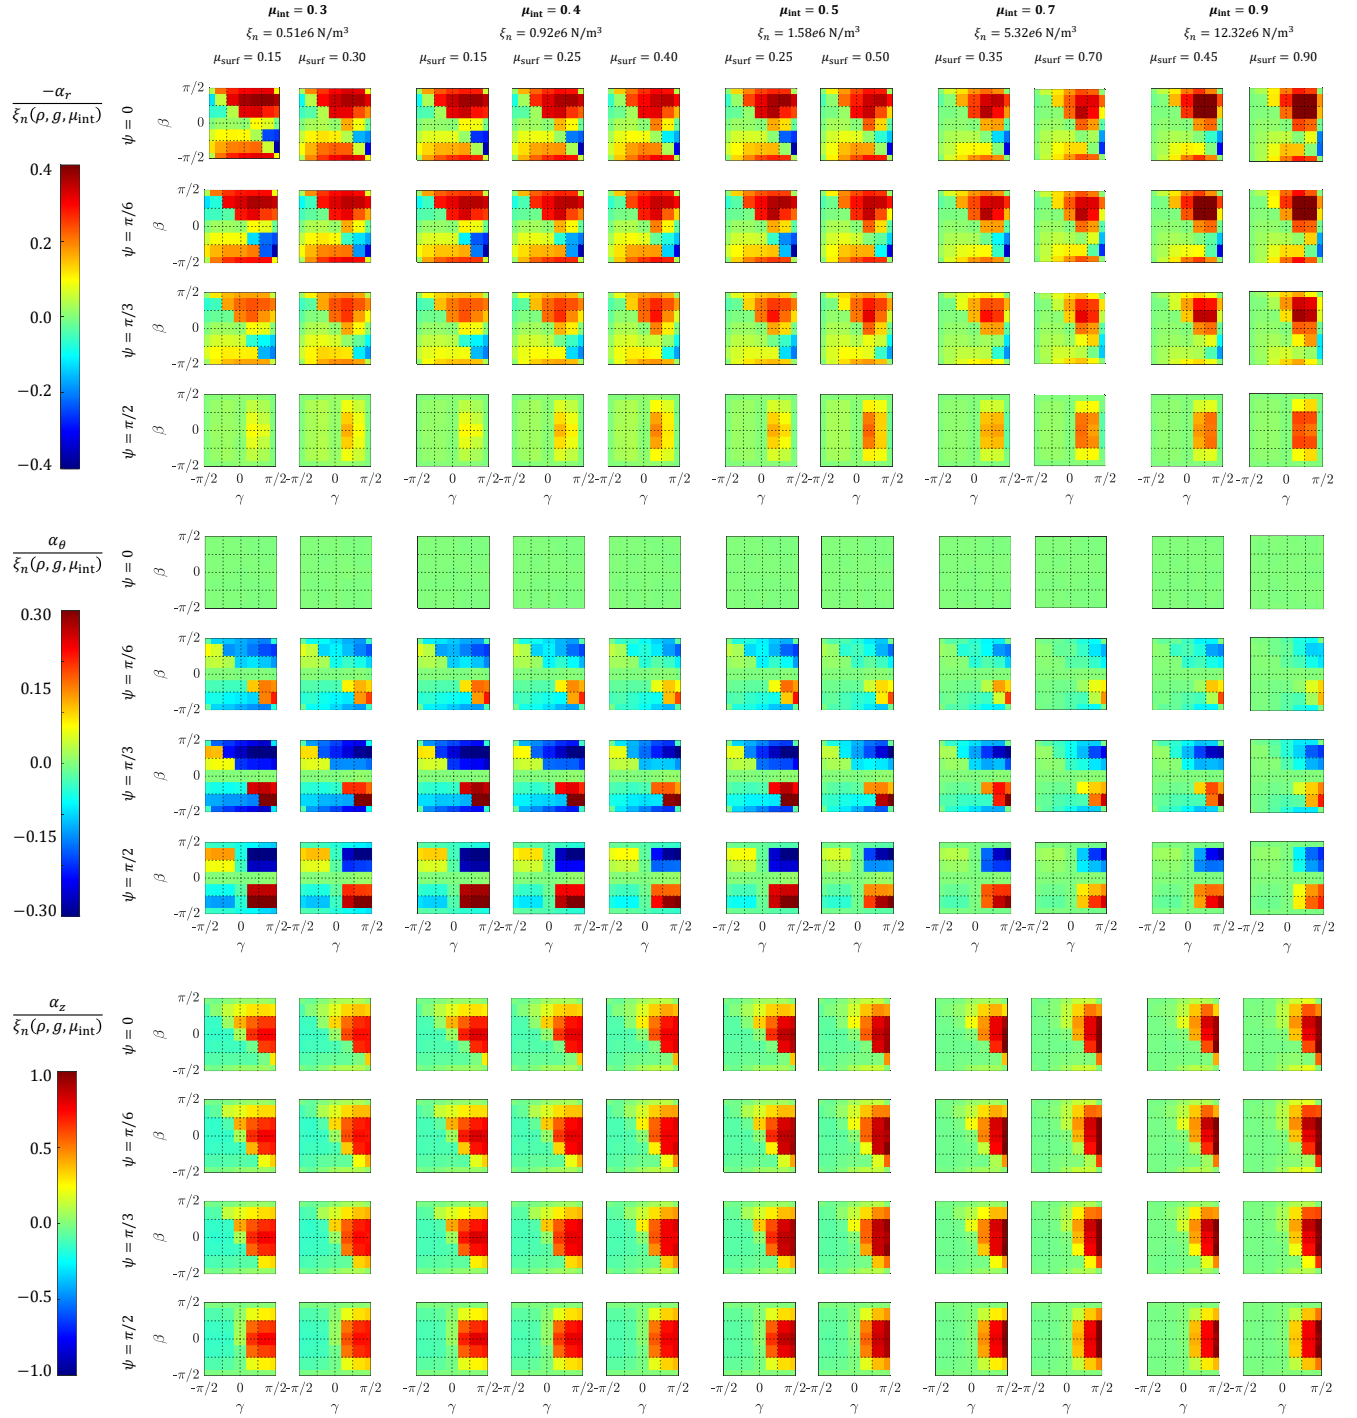

**Fig. S8. 3D-RFT Raw data:** Normalized  $\alpha_{r,\theta,z}$  value for 3D-RFT reference data used for generation of 3D-RFT form. Corresponding values of  $\mu_{\text{int}}$ ,  $\mu_{\text{surf}}$ , and  $\xi_n$  are written at the top of each column.

**Table S3.  $f_1, f_2, f_3$  3<sup>rd</sup> degree polynomial definitions**

$$f_i = \sum_k c_i^k T_k = c_i^1 + c_i^2 p_1 + \dots + c_i^{19} p_1 p_3^2 + c_i^{20} p_1 p_2 p_3$$

$$[p_1 \equiv \hat{\mathbf{g}} \cdot \hat{\mathbf{v}} = \sin \gamma, \quad p_2 \equiv \hat{\mathbf{g}} \cdot \hat{\mathbf{n}} = \cos \beta, \quad p_3 \equiv \hat{\mathbf{n}} \cdot \hat{\mathbf{v}} = \cos \psi \cos \gamma \sin \beta + \sin \gamma \cos \beta]$$

| $k$ | $T_k$         | $c_1^k$  | $c_2^k$  | $c_3^k$  |
|-----|---------------|----------|----------|----------|
| 1   | 1             | 0.00212  | -0.06796 | -0.02634 |
| 2   | $p_1$         | -0.02320 | -0.10941 | -0.03436 |
| 3   | $p_2$         | -0.20890 | 0.04725  | 0.45256  |
| 4   | $p_3$         | -0.43083 | -0.06914 | 0.00835  |
| 5   | $p_1^2$       | -0.00259 | -0.05835 | 0.02553  |
| 6   | $p_2^2$       | 0.48872  | -0.65880 | -1.31290 |
| 7   | $p_3^2$       | -0.00415 | -0.11985 | -0.05532 |
| 8   | $p_1 p_2$     | 0.07204  | -0.25739 | 0.06790  |
| 9   | $p_2 p_3$     | -0.02750 | -0.26834 | -0.16404 |
| 10  | $p_3 p_1$     | -0.08772 | 0.02692  | 0.02287  |
| 11  | $p_1^3$       | 0.01992  | -0.00736 | 0.02927  |
| 12  | $p_2^3$       | -0.45961 | 0.63758  | 0.95406  |
| 13  | $p_3^3$       | 0.40799  | 0.08997  | -0.00131 |
| 14  | $p_1 p_2^2$   | -0.10107 | 0.21069  | -0.11028 |
| 15  | $p_2 p_1^2$   | -0.06576 | 0.04748  | 0.01487  |
| 16  | $p_2 p_3^2$   | 0.05664  | 0.20406  | -0.02730 |
| 17  | $p_3 p_2^2$   | -0.09269 | 0.18519  | 0.10911  |
| 18  | $p_3 p_1^2$   | 0.01892  | 0.04934  | -0.04097 |
| 19  | $p_1 p_3^2$   | 0.01033  | 0.13527  | 0.07881  |
| 20  | $p_1 p_2 p_3$ | 0.15120  | -0.33207 | -0.27519 |

**Table S4.  $f_1, f_2$ , and  $f_3$  function definitions with 4<sup>th</sup> degree polynomials**

$$f_i = \sum_k c_i^k T_k = c_i^1 + c_i^2 p_1 + \dots + c_i^{19} p_1 p_3^2 + c_i^{35} p_1 p_2 p_3^2$$

$$[p_1 \equiv \hat{\mathbf{g}} \cdot \hat{\mathbf{v}} = \sin \gamma, \quad p_2 \equiv \hat{\mathbf{g}} \cdot \hat{\mathbf{n}} = \cos \beta, \quad p_3 \equiv \hat{\mathbf{n}} \cdot \hat{\mathbf{v}} = \cos \psi \cos \gamma \sin \beta + \sin \gamma \cos \beta]$$

| $k$ | $T_k$           | $c_1^k$  | $c_2^k$  | $c_3^k$  | $k$ | $T_k$           | $c_1^k$  | $c_2^k$  | $c_3^k$  |
|-----|-----------------|----------|----------|----------|-----|-----------------|----------|----------|----------|
| 1   | 1               | 0.00412  | -0.06300 | 0.00892  | 2   | $p_1$           | -0.02136 | -0.00336 | -0.03143 |
| 3   | $p_2$           | -0.21785 | -1.32520 | -0.54392 | 4   | $p_3$           | -0.54991 | 0.00048  | 0.01939  |
| 5   | $p_1^2$         | -0.03285 | -0.11116 | -0.11861 | 6   | $p_2^2$         | 0.87718  | 5.36790  | 2.03150  |
| 7   | $p_3^2$         | -0.00286 | 0.07983  | -0.13326 | 8   | $p_1 p_2$       | -0.38369 | 0.08966  | 0.47638  |
| 9   | $p_2 p_3$       | 0.48733  | -0.11872 | -0.35913 | 10  | $p_3 p_1$       | -0.16974 | 0.09029  | 0.13672  |
| 11  | $p_1^3$         | 0.01923  | -0.10024 | 0.01495  | 12  | $p_2^3$         | -1.82110 | -7.53640 | -2.44120 |
| 13  | $p_3^3$         | 0.71170  | -0.03393 | -0.01711 | 14  | $p_1 p_2^2$     | 1.03580  | -0.48634 | -1.14260 |
| 15  | $p_2 p_1^2$     | -0.06899 | 0.07279  | 0.20511  | 16  | $p_2 p_3^2$     | 0.01924  | 0.15943  | 0.01142  |
| 17  | $p_3 p_2^2$     | -1.58070 | -0.45871 | 0.52431  | 18  | $p_3 p_1^2$     | 0.07461  | 0.10419  | -0.03870 |
| 19  | $p_1 p_3^2$     | 0.04814  | -0.09860 | 0.10985  | 20  | $p_1 p_2 p_3$   | 0.05565  | -0.21270 | -0.06686 |
| 21  | $p_1^4$         | 0.02884  | -0.02951 | 0.11721  | 22  | $p_2^4$         | 1.10100  | 3.35300  | 0.90658  |
| 23  | $p_3^4$         | 0.03094  | -0.45255 | 0.03809  | 24  | $p_1^3 p_2$     | 0.24807  | 0.07722  | -0.25744 |
| 25  | $p_1^3 p_3$     | 0.05269  | -0.07405 | -0.26752 | 26  | $p_2^3 p_1$     | -0.72304 | 0.32683  | 0.67218  |
| 27  | $p_2^3 p_3$     | 1.15170  | 0.39561  | -0.31197 | 28  | $p_3^3 p_1$     | 0.20145  | -0.13273 | -0.11735 |
| 29  | $p_3^3 p_2$     | -0.09466 | 0.15479  | 0.06806  | 30  | $p_1^2 p_2^2$   | 0.12995  | 0.08606  | -0.12606 |
| 31  | $p_1^2 p_3^2$   | -0.06983 | 0.19846  | 0.18106  | 32  | $p_2^2 p_3^2$   | 0.09628  | 0.29711  | -0.02546 |
| 33  | $p_1^2 p_2 p_3$ | -0.57151 | -0.07567 | 0.54032  | 34  | $p_1 p_2^2 p_3$ | -0.24520 | -0.05941 | -0.06226 |
| 35  | $p_1 p_2 p_3^3$ | 0.03159  | 0.14051  | -0.33556 |     |                 |          |          |          |

## References

1. LK Treers, C Cao, HS Stuart, Granular resistive force theory implementation for three-dimensional trajectories. *IEEE Robotics Autom. Lett.* **6**, 1887–1894 (2021).
2. L Huang, J Zhu, Y Yuan, Y Yin, A dynamic resistive force model for designing mobile robot in granular media. *IEEE Robotics Autom. Lett.* **7**, 5357–5364 (2022).
3. H Askari, K Kamrin, Intrusion rheology in grains and other flowable materials. *Nat. materials* **15**, 1274–1279 (2016).
4. K Diaz, B Chong, S Tarr, E Erickson, DI Goldman, Water surface swimming dynamics in lightweight centipedes (2022).
5. CN Adkins, RH Liebeck, Design of optimum propellers. *J. Propuls. Power* **10**, 676–682 (1994).
6. J Gray, G Hancock, The propulsion of sea-urchin spermatozoa. *J. Exp. Biol.* **32**, 802–814 (1955).
7. W Kang, Y Feng, C Liu, R Blumenfeld, Archimedes' law explains penetration of solids into granular media. *Nat. communications* **9**, 1–9 (2018).

166 8. Hao Li , CSCI 599: Digital Geometry Processing, Differential operators on polygons (2015) <http://cs599.hao-li.com/>.
